# Supplementary material for: Egocentric Videoconferencing
Source: arXiv:2107.03109 source file (2021-07-07)
Supplement: Supplementary file 1 [file appendix.tex]

\appendix
\section{Appendix}

Tab.~1--2 lists the sequences used in our experiments. For each sequence, we indicate the total number of frames. We use 7,500 frames for training our technique, 2,500 frames for validation and the rest for testing.

\begin{table}[H]
	\newcommand{\subfig}[2][0px 0px 0px 0px]{\raisebox{-.3\height}{\includegraphics[width=20mm, trim=#1, clip]{IMAGES/#2}}}
	\caption{\label{tab:datasets}
		List of sequences used in our experiments.
	}
	
	\begin{tabular}{clclr}
	Image               & Name        & Type & Number of frames \\ \hline
    \subfig{jalees}    & ID1V1.       &   outdoor dynamic    &    13500 \\
    \subfig{mohamed}    & ID2V1.       &   outdoor dynamic    &    5700 \\
    \subfig{mohamed2}    & ID2V2.       &   outdoor dynamic    &    13640 \\
    \subfig{franzi}    & ID3.       &   indoor dynamic    &    13050 \\
    \subfig{vlad}    & ID4.       &   indoor dynamic    &    13450 \\
    \subfig{mohit1}    & ID5V1.       &   outdoor dynamic    &    12600 \\
    \subfig{mohit2c}    & ID5V2.       &   outdoor dynamic    &    14750 \\
    \subfig{mohit3}    & ID5V3.       &   outdoor dynamic    &    5796 \\
    \subfig{mohamed3}    & ID2V3.       &  sitting scenario    &    14500 \\
    \subfig{theobalt}    & ID6.       &   sitting scenario    &    13800 \\
    \subfig{ikhsi}    & ID7.       &   sitting scenario    &    14730 \\
    \subfig{mohit4}    & ID5V4.       &   sitting scenario    &    14700 \\
    \subfig{Gereon2}    & ID8V1.       &   sitting scenario    &    13500 \\
    \subfig{mbr}    & ID9.       &   sitting scenario    &    14260 \\
    \subfig{jalees2}    & ID1V2.       &   stress expressions    &    15600 \\
	 \subfig{Lingjie}    & ID10.       &   stress expressions    &    14500 \\
    \subfig{varshini}    & ID11.       &   stress expressions    &    14600 \\
     \subfig{vikram}    & ID12V1.       &   stress expressions    &    14740 \\
         \subfig{moritz}    & ID13.       &   stress expressions    &    14500 \\
	\end{tabular}
\end{table}

\begin{table}[H]
	\newcommand{\subfig}[2][0px 0px 0px 0px]{\raisebox{-.3\height}{\includegraphics[width=20mm, trim=#1, clip]{IMAGES/#2}}}
	\caption{\label{tab:datasets2}
		List of sequences used in our experiments.
	}
	
	\begin{tabular}{clclr}
	Image               & Name        & Type & Number of frames \\ \hline
    \subfig{Gereon}    & ID8V2.       &   stress expressions    &    13880 \\
    \subfig{mohit5}    & ID5V5.       &   stress expressions    &    14400 \\
    \subfig{vikram2}    & ID12V2.       &   outdoor dynamic    &    17300 \\
    \subfig{MH4}    & ID2V4.       &   sitting scenario    &    16000 \\ 
    \subfig{MH5}    & ID2V5.       &   stress expressions    &    16000 \\ 
    \subfig{M5}    & ID5V6.       &   sitting scenario    &    13000 \\
    \subfig{M6}    & ID5V7.       &   stress expressions    &    13000 \\
     \subfig{M7}   & ID5V8.       &   stress expressions    &    13000 \\
       \\
	\end{tabular}
\end{table}
